# Supplementary material for: GNNFlow: A Distributed Framework for Continuous Temporal GNN Learning on Dynamic Graphs
Source: arXiv:2311.17410 source file (2023-11-30)
Supplement: Supplementary file 1 [file appendix.tex]

\clearpage
